# Supplementary material for: Exponential Weights on the Hypercube in Polynomial Time
Source: arXiv:1806.04594 source file (2019-08-22)
Supplement: Supplementary file 1 [file suppliment.tex]

\section{Supplementary Proofs}
\subsection{Exp2 Regret Proofs}
First, we directly analyze Exp2's regret for the two kinds of feedback.
\subsubsection{Full Information}
\begin{lemma}\label{Lemma1}Let $L_t(X) = X^\top l_t$. If $|\eta L_t(X)| \leq 1$ for all $t \in [T]$ and $X \in \{0,1\}^n$, the Exp2 algorithm satisfies for any $X$:
$$\sum_{t=1}^T p_t^\top L_t - \sum_{t=1}^T L_t(X) \leq \eta \sum_{t=1}^T p_t^\top L_t^2 + \frac{n\log 2}{\eta}$$
\end{lemma}
\begin{proof}
(Adapted from \cite{hazan2016introduction} Theorem 1.5) Let $Z_{t} = \sum_{Y \in \{0,1\}^n}w_t(Y)$. We have:
\begin{align*}
Z_{t+1} &= \sum_{Y \in \{0,1\}^n}\exp(-\eta L_t(Y))w_t(Y)\\
&= Z_t \sum_{Y \in \{0,1\}^n}\exp(-\eta L_t(Y)) p_t(Y)
\end{align*}
Since $e^{-x} \leq 1-x+x^2$ for $x\geq -1$, we have that $\exp(-\eta L_t(Y)) \leq 1-\eta L_t(Y)+\eta^2 L_t(Y)^2$ (Because we assume $|\eta L_t(X)| \leq 1$). So,
\begin{align*}
Z_{t+1} &\leq Z_t \sum_{Y \in \{0,1\}^n}(1-\eta L_t(Y)+\eta^2 L_t(Y)^2) p_t(Y) \\
&= Z_t (1 - \eta p_t^\top L_t + \eta^2 p_t^\top L_t^2)
\end{align*}
Using the inequality $1+x \leq e^x$,
\begin{align*}
Z_{t+1} &\leq Z_t \exp( -\eta p_t^\top L_t + \eta^2 p_t^\top L_t^2)
\end{align*}
Hence, we have:
$$Z_{T+1} \leq Z_1 \exp( -\sum_{t=1}^T\eta p_t^\top L_t + \sum_{t=1}^T\eta^2 p_t^\top L_t^2)$$
For any $X \in \{0,1\}^n$, $w_{T+1}(X) = \exp(-\sum_{t=1}^T\eta L_t(X) )$. Since $w(T+1)(X) \leq Z_{T+1}$ and $Z_1 = 2^n$, we have:
\begin{align*}
\exp(-\sum_{t=1}^T\eta L_t(X) ) \leq 2^n \exp( -\sum_{t=1}^T\eta p_t^\top L_t + \sum_{t=1}^T\eta^2 p_t^\top L_t^2)
\end{align*}
Taking the logarithm on both sides manipulating this inequality, we get:
$$\sum_{t=1}^T p_t^\top L_t - \sum_{t=1}^T L_t(X) \leq \eta \sum_{t=1}^T p_t^\top L_t^2 + \frac{n\log 2}{\eta}$$
\end{proof}
\ExpFReg*
\begin{proof}
Using $L_t(X) = X^\top l_t$ and applying expectation with respect to the randomness of the player to definition of regret, we get:
\begin{align*}
E[\mathcal{R}_T] &= \sum_{t=1}^T \sum_{X \in \{0,1\}^n}p_t(X)L_t(X) - \min_{X^\star \in \{0,1\}^n}\sum_{t=1}^T L_t(X^\star) \\
&=  \sum_{t=1}^T p_t^\top L_t - \min_{X^\star \in \{0,1\}^n}\sum_{t=1}^T L_t(X^\star)
\end{align*}
Applying Lemma \ref{Lemma1}, we get $E[\mathcal{R}_T] \leq \eta \sum_{t=1}^T p_t^\top L_t^2 + n\log 2/\eta$. Since $|L_t(X)| \leq n $ for all $X  \in \{0,1\}^n$, we get $\sum_{t=1}^T p_t^\top L_t^2 \leq  T n^2 $.
$$E[\mathcal{R}_T] \leq \eta Tn^2 + \frac{n\log 2}{\eta}$$
Optimizing over the choice of $\eta$, we get the regret is bounded by $2n^{3/2} \sqrt{T \log 2}$ if we choose $\eta = \sqrt{\frac{\log 2}{nT}}$.

To apply Lemma \ref{Lemma1}, $|\eta L_t(X)| \leq 1$ for all $t \in [T]$ and $X \in \{0,1\}^n$. Since $|L_t(X)| \leq n$, we have $\eta \leq 1/n$.
\end{proof}
\subsubsection{Bandit}
\begin{lemma}\label{lemma5_1} Let $\tilde{L_t}(X) = X^\top \tilde{l}_t$, where $\tilde{l}_t = P_t^{-1}X_tX_t^\top l_t$. If $|\eta\tilde{L_t}(X)| \leq 1$ for all $t \in [T]$ and $X \in \{0,1\}^n$, the Exp2 algorithm with uniform exploration satisfies for any $X$
$$\sum_{t=1}^T  q_t^\top L_t - \sum_{t=1}^T L_t(X) \leq \eta \mathbb{E}[\sum_{t=1}^T q_t^\top \tilde{L}_t^2] + \frac{n\log 2}{\eta} + 2\gamma n T$$
\end{lemma}
\begin{proof}
We have that:
\begin{align*}
\sum_{t=1}^T q_t^\top \tilde{L}_t - \sum_{t=1}^T \tilde{L}_t(X)  &= (1-\gamma) (\sum_{t=1}^T p_t^\top \tilde{L}_t - \sum_{t=1}^T \tilde{L}_t(X)) \\&+ \gamma (\sum_{t=1}^T \mu^\top \tilde{L}_t - \sum_{t=1}^T \tilde{L}_t(X))
\end{align*}
Since the algorithm essentially runs Exp2 using the losses $\tilde{L}_t(X)$ and $|\eta\tilde{L_t}(X)| \leq 1$, we can apply Lemma \ref{Lemma1}:
\begin{align*}
\sum_{t=1}^T q_t^\top \tilde{L}_t - \sum_{t=1}^T \tilde{L}_t(X)  &\leq (1-\gamma) (\frac{n \log 2}{\eta} + \eta \sum_{t=1}^T p_t^\top \tilde{L}_t^2) \\&+ \gamma (\sum_{t=1}^T \mu^\top \tilde{L}_t - \sum_{t=1}^T \tilde{L}_t(X))
\end{align*}
Apply expectation with respect to $X_t$.  Using the fact that $\mathbb{E}[\tilde{l}_t] = l_t$ and $\mu^\top L_t -  L_t(X) \leq 2n$:
\begin{align*}
\sum_{t=1}^T q_t^\top L_t - \sum_{t=1}^T L_t(X)  &\leq (1-\gamma) (\frac{n \log 2}{\eta} + \eta \mathbb{E}[\sum_{t=1}^T p_t^\top \tilde{L}_t^2]) \\&+ \gamma (\sum_{t=1}^T \mu^\top L_t - \sum_{t=1}^T L_t(X))\\
&\leq \eta \mathbb{E}[\sum_{t=1}^T q_t^\top \tilde{L}_t^2] + \frac{n \log 2}{\eta}  + 2 \gamma nT
\end{align*}
\end{proof}
\ExpBanReg*
\begin{proof}
Applying expectation with respect to the randomness of the player to the definition of regret, we get:
\begin{align*}
\mathbb{E}[\mathcal{R}_T] &= \mathbb{E}[\sum_{t=1}^T L_t(X_t) - \min_{X^\star \in \{0,1\}^n} L_t(X^\star)] \\&= \sum_{t=1}^T  q_t^\top L_t - \min_{X^\star \in \{0,1\}^n}\sum_{t=1}^T L_t(X^\star)
\end{align*}
Applying Lemma \ref{lemma5_1}
$$\mathbb{E}[\mathcal{R}_T] \leq \eta \mathbb{E}[\sum_{t=1}^T q_t^\top \tilde{L}_t^2] + \frac{n \log 2}{\eta}  + 2 \gamma nT$$
We follow the proof technique of \cite{bubeck2012towards} Theorem 4. We have that:
\begin{align*}
q_t^\top \tilde{L}_t^2 &= \sum_{X \in \{0,1\}^n}q_t(X)(X^\top \tilde{l_t})^2  \\&= \sum_{X \in \{0,1\}^n}q_t(X)(\tilde{l_t}^\top X X^\top \tilde{l_t})\\
&= \tilde{l_t}^\top P_t \tilde{l_t} \\&= l_t^\top X_tX_t^\top P_t^{-1}  P_t P_t^{-1}X_t X_t^\top l_t \\&= (X_t^\top l_t)^2 X_t^\top P_t^{-1}X_t\\
&\leq n^2 X_t^\top P_t^{-1}X_t = n^2 \text{Tr}(P_t^{-1} X_t X_t^\top )
\end{align*}
Taking expectation, we get $E[q_t^\top \tilde{L}_t^2] \leq n^2 \text{Tr}(P_t^{-1} \mathbb{E}[X_t X_t^\top] )= n^2 \text{Tr}(P_t^{-1} P_t) = n^3$.
Hence,
$$\mathbb{E}[\mathcal{R}_T] \leq \eta n^3 T + \frac{n \log 2}{\eta}  + 2 \gamma nT$$
However, in order to apply Lemma \ref{lemma5_1}, we need that $|\eta X^\top \tilde{l}_t| \leq 1$. We have that
$$|\eta X^\top \tilde{l}_t| = \eta |(X_t ^\top l_t) X^\top P_t^{-1} X_t| \leq 1$$
As $|X_t ^\top l_t| \leq n$ and $|X_t^\top X|\leq n$, we get $\eta n |X^\top P_t^{-1} X_t|  \leq \eta n |X^\top X_t|\|P_t^{-1}\|\leq \eta n^2\|P_t^{-1}\| \leq 1 $. The matrix $P_t = (1-\gamma)\Sigma_t + \gamma \Sigma_\mu$. The smallest eigenvalue of $\Sigma_\mu$ is $1/4$\cite{cesa2012combinatorial}. So $P_t \succeq \frac{\gamma}{4} I_n $ and $P_t^{-1} \preceq \frac{4}{\gamma}I_n$. We should have that $\frac{4n^2 \eta}{\gamma}\leq 1$. Substituting $\gamma = 4n^2 \eta$ in the regret inequality, we get:
\begin{align*}
\mathbb{E}[\mathcal{R}_T] &\leq \eta n^3 T + 8\eta n^3 T +  \frac{n \log 2}{\eta}\\
&\leq 9\eta n^3T +  \frac{n \log 2}{\eta}
\end{align*}
Optimizing over the choice of $\eta$, we get $\mathbb{E}[\mathcal{R}_T] \leq 2 n^{2} \sqrt{9T \log 2}$ when $\eta = \sqrt{\frac{\log 2}{9n^2T}}$.
\end{proof}

\subsection{Lower Bounds}
\subsubsection{Full Information Lower bound}

In the game between player and adversary, the players strategy is to pick some probability distribution $p_t \in \Delta(\{0,1\}^n)$ for $t=1\dots T$. The adversary picks a density $q_t$ over loss vectors $l \in [-1,1]^n$ for $t=1 \dots T$. So player picks $X_t \sim p_t$ and adversary picks $l_t \sim q_t$.  The min max expected regret is:
$$\inf_{p_1 \dots p_T} \sup_{q_1 \dots q_t}   \mathbb{E}_{l_t \sim q_t} \mathbb{E}_{X_t \sim p_t}\left[\sum_{t=1}^T l_t^\top X_t - \min_X \sum_{t=1}^T l_t^\top X  \right] $$
Let $\mathbb{E}_{X_t \sim p_t} = x_t$. 
$$\inf_{p_1 \dots p_T} \sup_{q_1 \dots q_t} \mathbb{E}_{l_t \sim q_t} [\sum_{t=1}^T l_t^\top x_t - \min_X \sum_{t=1}^T l_t^\top X] $$

\LBFull*

\begin{proof}
We choose $q_t$ to be the density such that $l_{t,i}$ is a Rademacher random variable, ie, $l_{t,i} = +1$ w.p. $1/2$ and $l_{t,i}=-1$ w.p $1/2$ for all $t=1\dots T$ and $i=[n]$. So,
\begin{align*}
    &\inf_{p_1 \dots p_T} \sup_{q_1 \dots q_t} \mathbb{E}_{l_t \sim q_t} \left[\sum_{t=1}^T l_t^\top x_t - \min_X \sum_{t=1}^T l_t^\top X   \right] \\&\geq \inf_{p_1 \dots p_T} \mathbb{E}_{l_{t}} \left[\sum_{t=1}^T l_t^\top x_t - \min_X \sum_{t=1}^T l_t^\top X  \right]
\end{align*}
For our choice of $q_t$, we have $\mathbb{E}_{l_{t}} [l_t^\top x_t] = 0$. So,
\begin{align*}
    &\inf_{p_1 \dots p_T} \mathbb{E}_{l_{t}} [\sum_{t=1}^T l_t^\top x_t - \min_X \sum_{t=1}^T l_t^\top X] \\&= \inf_{p_1 \dots p_T} \mathbb{E}_{l_{t}} [- \min_X \sum_{t=1}^T l_t^\top X] \\
    &= \mathbb{E}_{l_{t}} [\max_X \sum_{t=1}^T l_t^\top X]
\end{align*}

Simplifying this, we get:
\begin{align*}
        \mathbb{E}_{l_{t}} [\max_X \sum_{t=1}^T l_t^\top X] &= \mathbb{E}_{l_{t}} [\max_{X_1\dots X_n} \sum_{t=1}^T \sum_{i=1}^n l_{t,i} X_i]\\
        &= \mathbb{E}_{l_{t}}[\sum_{i=1}^n\max_{X_i} \sum_{t=1}^T  l_{t,i} X_i]\\
        &= \sum_{i=1}^n \mathbb{E}_{l_{t,i}}[\max_{X_i} \sum_{t=1}^T  l_{t,i} X_i]\\
        &= n \mathbb{E}_{Y}[\max_{x} \sum_{t=1}^T  Y_{t} x]
\end{align*}
Here $Y$ is a Rademacher random vector of length $T$ and $x \in \{0,1\}$. We have that
$$\max_{x} \left[\sum_{t=1}^T  Y_{t} x\right] =\begin{cases} 0 \quad \text{ If } \sum_{t=1}^T  Y_{t} \leq 0 \\ \sum_{t=1}^T  Y_{t} \quad \text{ otherwise}
\end{cases}$$
So
\begin{align*}
    \mathbb{E}_{Y}\left[\max_{x} \sum_{t=1}^T  Y_{t} x  \right] &= \mathbb{E}_{Y}[\sum_{t=1}^T  Y_{t} | \sum_{t=1}^T  Y_{t} >0]\\
    &= \frac{1}{2}\mathbb{E}_{Y}  \left| {\sum_{t=1}^T  Y_{t}} \right|  
\end{align*}
Using Khintchine's inequality, we have positive constants $A$ and $B$ such that:
$$A\left( \sum _ { t = 1 } ^ { T } \left|1 \right| ^ { 2 } \right) ^ { 1 / 2 } \leq \mathbb{E}_{Y}  \left| {\sum_{t=1}^T  Y_{t}} \right| \leq B\left( \sum _ { t = 1 } ^ { T } \left|1 \right| ^ { 2 } \right) ^ { 1 / 2 }$$
Hence, the regret is lower bounded by $\Omega(n \sqrt{T})$.
\end{proof}
\subsubsection{Bandit Lower bound}
\LBBandit*
\begin{proof}
We consider $2^n$ stochastic adversaries indexed by $X \in \{0,1\}^n$. Adversary $X$ draws losses as follows:
\begin{equation*}
    l_{t,i} = \begin{cases} \begin{cases} +1 \text{ w.p } \frac{1}{2}+\epsilon\\
    -1 \text{ w.p } \frac{1}{2}-\epsilon
    \end{cases} \text{ if } X_i = 0\\
    \begin{cases} +1 \text{ w.p } \frac{1}{2} - \epsilon\\
    -1 \text{ w.p } \frac{1}{2} + \epsilon
    \end{cases} \text{ if } X_i = 1
    \end{cases}
\end{equation*}
Let $\tilde{l}_{t} = [X_1^\top l_1,X_2^\top l_2,\dots,X_t^\top l_t]$. We consider deterministic algorithms, ie $X_t$ is a deterministic function of $\tilde{l}_{t-1}$. So, the only the adversary's randomness remains. The obtained result can be extended to randomized algorithms via application of Fubini's Theorem. Let $E_X$ denote the expectation conditioned on adversary $X$. When playing against adversary $X$, the vector $X$ is the best action in expectation. The expected regret when playing against adversary $X$.
\begin{align*}
    \mathbb{E}_X[\mathcal{R}_T] &= \mathbb{E}_X \left[ \sum_{t=1}^T l_t^\top X_t - \min_{X^\star}\sum_{t=1}^T l_t^\top X^\star\right]\\
    &\geq \mathbb{E}_X \left[ \sum_{t=1}^T l_t^\top X_t - \sum_{t=1}^T l_t^\top X\right]\\
    &= 2\epsilon \sum_{i=1}^n \mathbb{E}_X[\sum_{t=1}^T \textbf{1}(X_{i,t} \neq X_i)]\\
    &= 2\epsilon T \sum_{i=1}^n \left(1- \frac{\mathbb{E}_X[\sum_{t=1}^T \textbf{1}(X_{i,t} = X_i)]}{T} \right)
\end{align*}
$\sum_{t=1}^T \textbf{1}(X_{i,t} = X_i)/T$ is the empirical mean of playing $X_i$. Let $J_i$ be a Bernoulli random drawn according to this mean. Hence,
$$\mathbb{E}_X[\mathcal{R}_T] \geq 2\epsilon T \sum_{i=1}^n \left(1- \mathbb{P}_X(J_i=X_i) \right)$$
Taking the average over adversaries:
\begin{align*}
    \mathbb{E}[\mathcal{R}_T] &= \frac{1}{2^n}\sum_{X} \mathbb{E}_X[\mathcal{R}_T]\\
    &\geq 2\epsilon T \sum_{i=1}^n \left(1- \frac{1}{2^n}\sum_{X}\mathbb{P}_X(J_i=X_i) \right)
\end{align*}
Let $X^{\oplus i}$ be the vector $X$ with the $i$'th bit flipped. Using Pinsker's inequality, we have that:
$$\mathbb{P}_X(J_i = X_i) \leq \mathbb{P}_{X^{\oplus i}}(J_i = X_i) + \sqrt{\frac{1}{2}KL(\mathbb{P}_{X^{\oplus i}}\| \mathbb{P}_X)}$$
Taking the summation, and using the concavity of square root:
$$\frac{1}{2^n}\sum_{X} \mathbb{P}_X(J_i = X_i) \leq \frac{1}{2} + \sqrt{\frac{1}{2}\frac{1}{2^n}\sum_{X}KL(\mathbb{P}_{X^{\oplus i}}\| \mathbb{P}_X)}$$

The sequence of observed losses $\tilde{l}_{T} \in \{-n,\dots,+n\}^T$ determines the empirical distribution of plays. Let $\mathbb{P}^T_X$ be the law of $\tilde{l}_{T}$ when playing against adversary $X$. So, using the chain rule of Kullback Leibler divergence:
\begin{align*}
    &KL(\mathbb{P}_{X^{\oplus i}}\| \mathbb{P}_X)\leq KL(\mathbb{P}^T_{X^{\oplus i}}\| \mathbb{P}^T_X)  \\
    &=KL(\mathbb{P}^1_{X^{\oplus i}}\| \mathbb{P}^1_X) \\&+ \sum _ { t = 2 } ^ { T } \sum_{ \tilde{l} _ {t - 1 }  } \mathbb{P}^{t-1}_{X^{\oplus i}}(\tilde{l} _ { t - 1 })  KL(\mathbb{P}^t_{X^{\oplus i}}(\cdot|\tilde{l} _ { t - 1 })\| \mathbb{P}^t_X((\cdot|\tilde{l} _ {t - 1 }))\\
    &= KL(\mathcal{B}_{0}\|\mathcal{B'}_0) \textbf{1}(X_{1,i} = X_i) \\
    &+  \sum _ { t = T } ^ { t } \sum_{ \tilde{l} _ {t - 1 }:X_{t,i} = X_i  } \mathbb{P}^{t-1}_{X^{\oplus i}}(\tilde{l} _ { t - 1 })KL(\mathcal{B}_{\tilde{l}_{t-1}}\|\mathcal{B'}_{\tilde{l}_{t-1}})
\end{align*}
Here, $\mathcal{B}_{\tilde{l}_{t-1}},\mathcal{B'}_{\tilde{l}_{t-1}}$ are sums of at most $n$ Bernoulli random variables such that their means agree on all coordinates except $i$.
Using Lemma 24 from \cite{audibert2011minimax}, we get that:
$$KL(\mathcal{B}_{\tilde{l}_{t-1}}\|\mathcal{B'}_{\tilde{l}_{t-1}}) \leq \frac{16\epsilon^2}{ n }$$
Substituting this back into the previous expression, we get:
\begin{align*}
    KL(\mathbb{P}_{X^{\oplus i}}\| \mathbb{P}_X) &\leq \frac{16\epsilon^2}{n} \sum_{t=1}^T \sum_{\tilde{l}_{1:t-1} : X_{t,i}=X_i}\mathbb{P}^t_{X^{\oplus i}}(\tilde{l}_{1:t-1})\\
    &\leq \frac{16\epsilon^2}{n} \sum_{t=1}^T \mathbb{E}_{X^{\oplus i}}(\textbf{1}(X_{i,t}=X_i))\\
    &= \frac{16\epsilon^2}{n} T \mathbb{P}_{X^{\oplus i}}(J_i = X_i)
\end{align*}
Taking the summation, we have:
\begin{align*}
    \frac{1}{2^n} \sum_X KL(\mathbb{P}_{X^{\oplus i}}\| \mathbb{P}_X) \leq \frac{8\epsilon^2}{n} T 
\end{align*}
Substituting this in the regret inequality:
\begin{align*}
    \mathbb{E}[\mathcal{R}_T]&\geq 2\epsilon T \sum_{i=1}^n \left( 1- \frac{1}{2} - \sqrt{\frac{4 \epsilon^2 T}{n}}\right)\\
    &= 2\epsilon T n \left(\frac{1}{2} - 2 \epsilon\sqrt{\frac{T}{n}}\right)
\end{align*}
Optimizing over $\epsilon$, we get that $\mathbb{E}[\mathcal{R}_T] = \Omega(n^{3/2}\sqrt{T})$
\end{proof}

\subsection{$\{-1,+1\}^n$ Hypercube Case}
\begin{lemma} \label{lemma6}Exp2 on $\{-1,+1\}^n$ with losses $l_t$ is equivalent to Exp2 on $\{0,1\}^n$ with losses $2l_t$ while using the map $2X_t-\textbf{1}$ to play on $\{-1,+1\}^n$.
\end{lemma}
\begin{proof}
Consider the update equation for Exp2 on $\{-1,+1\}^n$
$$p_{t+1}(Z) = \frac{\exp(-\eta \sum_{\tau=1}^t Z^\top l_\tau)}{\sum_{W \in \{-1,+1\}^n}\exp(-\eta \sum_{\tau=1}^t W^\top l_\tau)}$$
$Z \in \{-1,+1\}^n$ can be mapped to a $X \in \{0,1\}^n$ using the bijective map $X = (Z+\textbf{1})/2$. So:
\begin{align*}
p_{t+1}(Z) &= \frac{\exp(-\eta \sum_{\tau=1}^t (2X-\textbf{1})^\top l_\tau)}{\sum_{Y \in \{0,1\}^n}\exp(-\eta \sum_{\tau=1}^t (2Y-\textbf{1})^\top l_\tau)}\\
&= \frac{\exp(-\eta \sum_{\tau=1}^t X^\top (2l_\tau))}{\sum_{Y \in \{0,1\}^n}\exp(-\eta \sum_{\tau=1}^t Y^\top (2l_\tau))}
\end{align*}
This is equivalent to updating the Exp2 on $\{0,1\}^n$ with the loss vector $2l_t$.
\end{proof}
\Hypereq*
\begin{proof}
After sampling $X_t$, we play $Z_t = 2X_t-\textbf{1}$. So $\Pr(X_t=X) = \Pr(Z_t = 2X -\textbf{1})$. In full information, $2\tilde{l}_t = 2l_t$ and in the bandit case $\mathbb{E}[2\tilde{l}_t] = 2l_t$. Since $2\tilde{l}_t$ is used to update the algorithm, by Lemma \ref{lemma6} we have that $\Pr(X_{t+1}=X) = \Pr(Z_{t+1} = 2X -\textbf{1})$. By equivalence of Exp2 to PolyExp, the first statement follows immediately. Let $Z^\star = \min \limits_{Z \in \{-1,+1\}^n} \sum_{t=1}^T Z^\top l_t$ and $2X^\star = Z^\star + \textbf{1}$. The regret of Exp2 on $\{-1,+1\}^n$ is:
\begin{align*}
\sum_{t=1}^T l_t^\top (Z_t - Z^\star) &= \sum_{t=1}^T l_t^\top (2X_t -\textbf{1} - 2X^\star + \textbf{1})\\&= \sum_{t=1}^T (2l_t)^\top (X_t - X^\star)
\end{align*}
\end{proof}
